# Supplementary material for: On the rank-reduced relativistic coupled cluster method
Source: arXiv:2506.21133 ancillary file (2025-06-26)
Supplement: Supplementary file 1 [file supplementary_materials.pdf]

# Supplementary: On the rank-reduced relativistic coupled cluster method

Alexander V. Oleynichenko,[1,2] Artem S. Rumiantsev,[1,3] Andréi Zaitsevskii,[1,4] and Ephraim Eliav[5]

[1] *Petersburg Nuclear Physics Institute named by B.P. Konstantinov of National Research Centre “Kurchatov Institute”, Orlova roshcha 1, Gatchina, Leningradskaya Oblast, 188300, Russia*

[2] *Moscow Center for Advanced Studies, 20 Kulakova Str., 123592 Moscow, Russia*

[3] *Saint Petersburg State University, 7/9 Universitetskaya nab., 199034 St. Petersburg, Russia*

[4] *Department of Chemistry, M. V. Lomonosov Moscow State University, 119991 Moscow, Russia*

[5] *School of Chemistry, Tel Aviv University, Tel Aviv 6997801, Israel*

## ADDITIONAL FIGURES

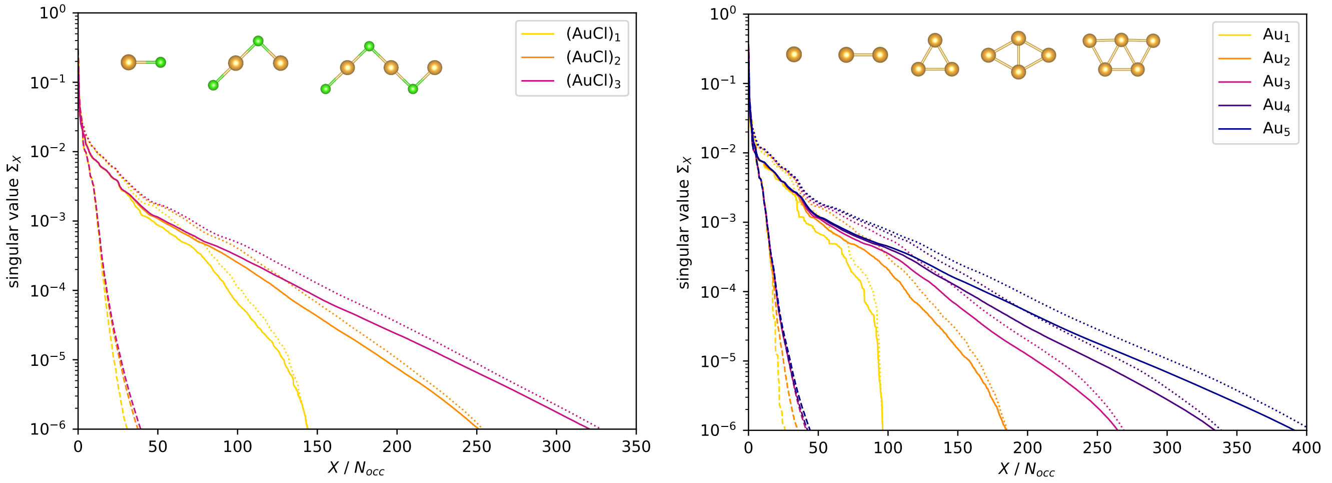


FIG. S1. Singular value distributions for the $t_{ij}^{ab}$ amplitude tensor obtained within the MP2 (dashed lines), MP3 (dotted lines) and CCSD (solid lines) approximations for (a) $(AuCl)_n$ chains, (b) $Au_n$ clusters. $\Sigma_X$ denotes singular values (cf. Eq. (9)). $X$ stands for the singular value index (singular values are sorted in the descending order). $X$ is divided by $N_{occ}$ which is proportional to the system size to make possible the direct comparison of distributions for different molecules.

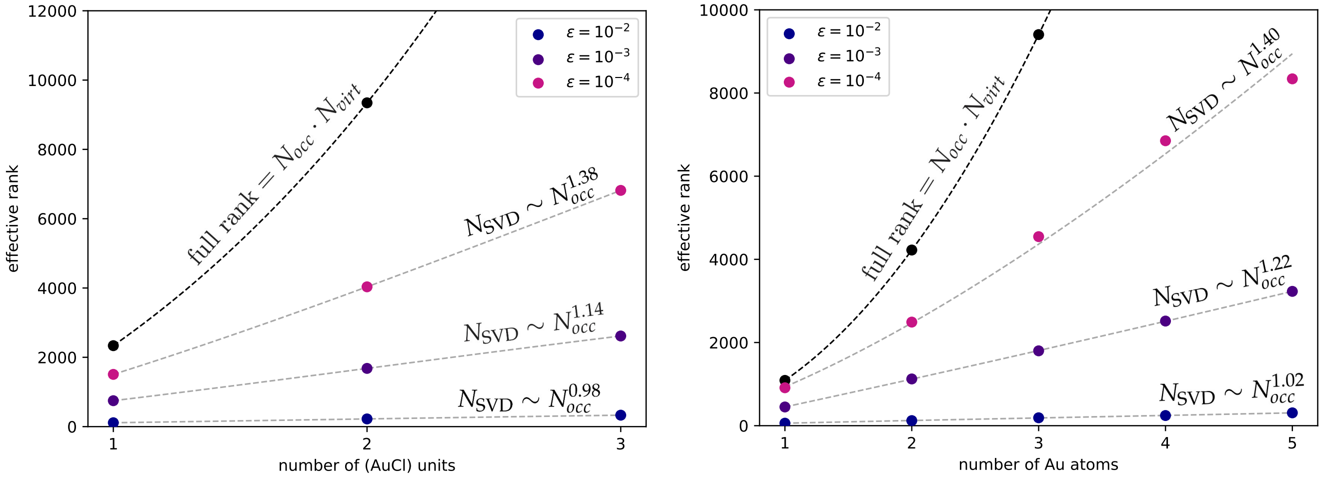


FIG. S2. Effective rank $N_{\mathrm{SVD}}$ of the $t_{ij}^{ab}$ amplitude tensor for different singular value thresholds $\varepsilon$ for (a) $(AuCl)_n$ chains, (b) $Au_n$ clusters. Full rank of a tensor equals to $N_{occ}N_{virt}$.

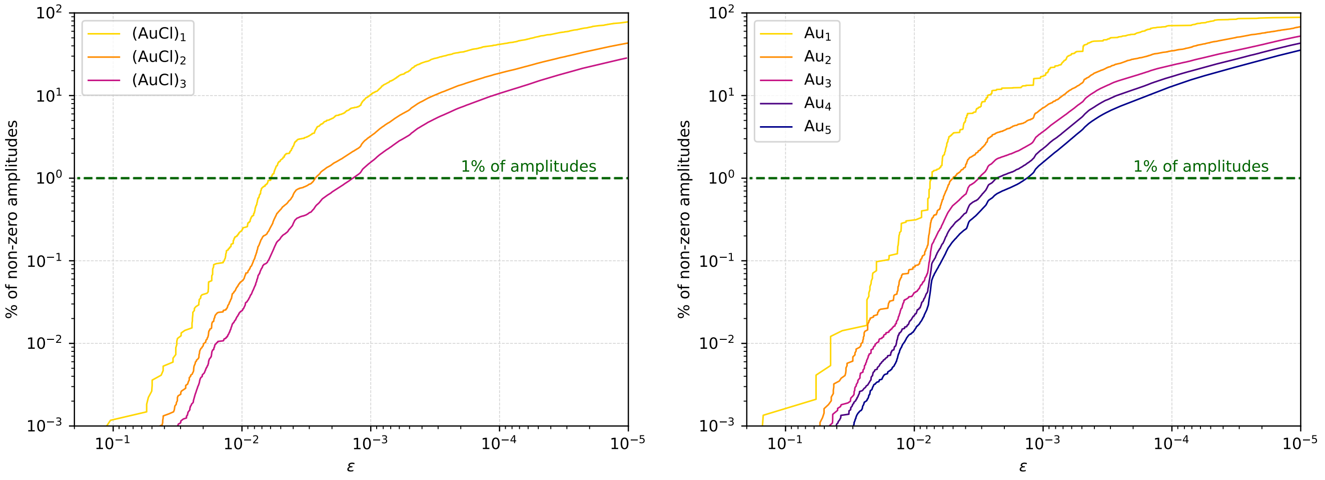


FIG. S3. Percentage of retained $t_{ij}^{ab}$ amplitudes with respect to the singular value threshold $\varepsilon$ for (a) $(AuCl)_n$ chains, (b) $Au_n$ clusters.

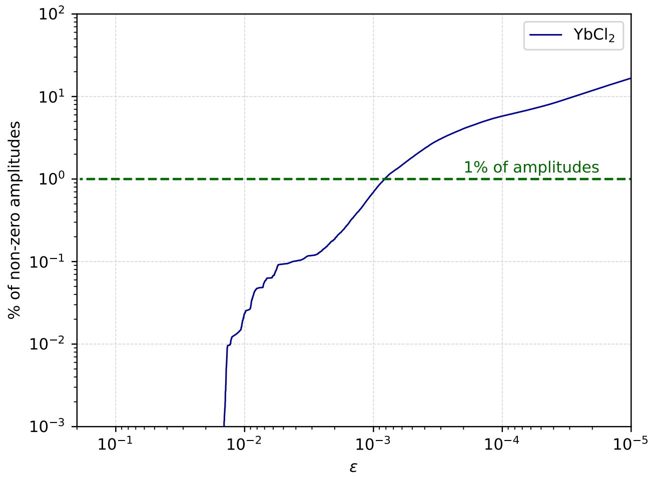


FIG. S4. Percentage of retained $t_{ij}^{ab}$ amplitudes with respect to the singular value threshold $\varepsilon$ for the cluster model of solid $YbCl_2$.

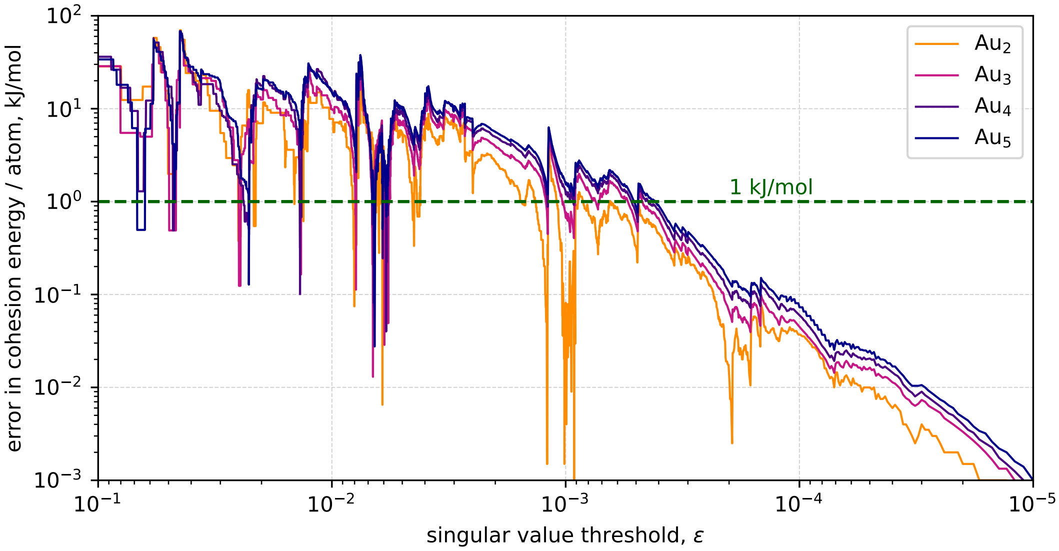


FIG. S5. Errors in cohesion energies of $Au_n$ clusters (kJ/mol, per 1 atom) with respect to the singular value threshold $\varepsilon$. The horizontal green dashed line marks the 1 kJ/mol accuracy threshold. Sharp variations of the error in cohesion energies are supposed to be caused by a non-monotonicity of correlation energies as functions of a threshold related to the non-variational nature of the coupled cluster energy estimates.

| System | $N_{occ}$ | $N_{virt}$ | $N$ |
|---|---|---|---|
| Au | 11 | 99 | 110 |
| $Au_2$ | 22 | 192 | 214 |
| $Au_3$ | 33 | 285 | 318 |
| $Au_4$ | 44 | 378 | 422 |
| $Au_5$ | 55 | 471 | 526 |
| | | | |
| AuCl | 16 | 146 | 162 |
| $(AuCl)_2$ | 32 | 292 | 324 |
| $(AuCl)_3$ | 48 | 436 | 484 |
| | | | |
| $YbCl_7$@CTEP | 42 | 512 | 554 |

TABLE I. Numbers of occupied ($N_{occ}$) and virtual ($N_{virt}$) spinors and the total number of spinors ($N$) for the systems considered in the present study.

## FACTORIZATION OF TERMS IN THE RR-CCD RESIDUAL EQUATIONS

The right-hand side of the residual equations for the relativistic RR-CCD method is obtained by projection of the expression $r_{ij}^{ab}$ onto the subspace of the compressed amplitudes by multiplication by $U_{ai}^{X*}U_{bj}^{Y*}$ and summing over the $i, j, a, b$ indices. (Equations for RR-CCSD are virtually the same except for the increased number of terms.) Here we also use the DF approximation to the tensor of two-electron integrals, i. e.

$$\langle pq|rs\rangle = (pr|qs) \approx \sum_Q B_{pr}^Q B_{qs}^Q.$$

Taking into account the cumbersomeness of the formulas, it is assumed that the summation is based on repeated indexes on the right side. Terms are named according to the book [1].

### Intermediate terms

$$O_{kilj} = B_{kc}^Q U_{ci}^{X'} T_{X'Y'} B_{ld}^Q U_{dj}^{Y'} = \sum_{RW}^{N_\mathrm{O}} \alpha_{ki}^R o^{RW} \alpha_{lj}^W,$$

where $\alpha_{ki}^R$ is the projector, and $o^{RW}$ is the core of the decomposition, $N_\mathrm{O}$ stands for the effective tensor rank of $O_{ki,lj}$.

$$o^{RW} = (B_{kc}^Q \alpha_{ki}^{R*} U_{ci}^{X'})(B_{ld}^Q \alpha_{lj}^{W*} U_{dj}^{Y'})T_{X'Y'}$$

$$Z_{kjbc} = B_{kd}^Q U_{dj}^{X''} T_{X''Y''} B_{lc}^Q U_{bl}^{Y''} = \sum_{FG}^{N_\mathrm{Z}} \beta_{kj}^F z^{FG} \beta_{bc}^G,$$

where $\beta_{kj}^F$ is the left projector, $\beta_{bc}^G$ is the right projector, and $z^{FG}$ is the core of the decomposition, $N_\mathrm{Z}$ stands for the effective tensor rank of $Z_{kj,bc}$.

$$z^{FG} = (B_{kd}^Q \beta_{kj}^{F*} U_{dj}^{X''})(B_{lc}^Q \beta_{bc}^{G*} U_{bl}^{Y''})T_{X'Y'}$$

### Terms of RR-CCD amplitude equations

D1 :
$$\begin{aligned} &U_{ai}^{X*}U_{bj}^{Y*}(ai|bj) = \\ &U_{ai}^{X*}B_{ai}^Q U_{bj}^{Y*}B_{bj}^Q \end{aligned} \qquad O(N_\mathrm{virt}N_\mathrm{occ}N_\mathrm{DF}N_\mathrm{SVD})$$

D2a :
$$\begin{aligned} U_{ai}^{X*}U_{bj}^{Y*}P(ai|bj)f_{ac}t_{ci}^{bj} &= \\ P(X|Y)U_{ai}^{X*}U_{bj}^{Y*}f_{ac}U_{bj}^{Y'}U_{ci}^{X'}T_{X'Y'} &= \\ P(X|Y)U_{ai}^{X*}U_{ci}^{X'}f_{ac}T_{X'Y} & \end{aligned} \qquad \begin{aligned} O(N_\mathrm{virt}^2 N_\mathrm{occ}N_\mathrm{SVD} \\ +N_\mathrm{virt}N_\mathrm{occ}N_\mathrm{SVD}^2 \\ +N_\mathrm{SVD}^3) \end{aligned}$$

D2b :
$$\begin{aligned} -U_{ai}^{X*}U_{bj}^{Y*}P(ai|bj)f_{ki}t_{ci}^{bj} &= \\ -P(X|Y)U_{ai}^{X*}U_{ak}^{X'}f_{ki}T_{X'Y} & \end{aligned} \qquad \begin{aligned} O(N_\mathrm{virt}N_\mathrm{occ}^2 N_\mathrm{SVD} \\ +N_\mathrm{virt}N_\mathrm{occ}N_\mathrm{SVD}^2 \\ +N_\mathrm{SVD}^3) \end{aligned}$$

D2c :
$$\begin{aligned} U_{ai}^{X*}U_{bj}^{Y*}(ac|bd)t_{ci}^{dj} &= \\ U_{ai}^{X*}U_{bj}^{Y*}B_{ac}^Q B_{ac}^Q U_{dj}^{Y'}U_{ci}^{X'}T_{X'Y'} &= \\ (U_{ai}^{X*}U_{ci}^{X'}B_{ac}^Q)(U_{bj}^{Y*}U_{dj}^{Y'}B_{bd}^Q)T_{X'Y'} & \end{aligned} \qquad \begin{aligned} O(2N_\mathrm{virt}^2 N_\mathrm{occ}N_\mathrm{SVD}N_\mathrm{DF} \\ +2N_\mathrm{virt}N_\mathrm{occ}N_\mathrm{SVD}^2 N_\mathrm{DF} \\ +2N_\mathrm{SVD}^3 N_\mathrm{DF}) \end{aligned}$$

D2d :

$$U_{ai}^{X*}U_{bj}^{Y*}(ki|lj)t_{ak}^{bl} = U_{ai}^{X*}U_{bj}^{Y*}B_{ki}^{Q}B_{lj}^{Q}U_{bl}^{Y'}U_{ak}^{X'}T_{X'Y'} = (U_{ai}^{X*}U_{ak}^{X'}B_{ki}^{Q})(U_{bj}^{Y*}U_{bl}^{Y'}B_{lj}^{Q})T_{X'Y'}$$

$$O(2N_{\mathrm{occ}}^2N_{\mathrm{virt}}N_{\mathrm{SVD}}^2 +2N_{\mathrm{occ}}^2N_{\mathrm{SVD}}^2N_{\mathrm{DF}} +2N_{\mathrm{SVD}}^3N_{\mathrm{DF}})$$

D2e(1) :

$$U_{ai}^{X*}U_{bj}^{Y*}(kc|bj)t_{ai}^{ck} = U_{ai}^{X*}U_{bj}^{Y*}B_{kc}^{Q}B_{bj}^{Q}U_{ck}^{Y'}U_{ai}^{X'}T_{X'Y'} = (U_{ck}^{Y'}B_{kc}^{Q})(U_{bj}^{Y*}B_{bj}^{Q})T_{XY'}$$

$$O(2N_{\mathrm{virt}}N_{\mathrm{occ}}N_{\mathrm{SVD}}N_{\mathrm{DF}} +2N_{\mathrm{DF}N_{\mathrm{SVD}}^2})$$

D2e(2) :

$$-U_{ai}^{X*}U_{bj}^{Y*}(kj|bc)t_{ai}^{ck} = -U_{ai}^{X*}U_{bj}^{Y*}B_{kj}^{Q}B_{bc}^{Q}U_{ck}^{Y'}U_{ai}^{X'}T_{X'Y'} = -(U_{ck}^{Y'}B_{kj}^{Q})(U_{bj}^{Y*}B_{bc}^{Q})T_{XY'}$$

$$O(2N_{\mathrm{virt}}N_{\mathrm{occ}}^2N_{\mathrm{SVD}}N_{\mathrm{DF}} +N_{\mathrm{virt}}N_{\mathrm{occ}}N_{\mathrm{DF}}N_{\mathrm{SVD}}^2 +N_{\mathrm{SVD}}^3)$$

D2e(3) :

$$U_{ai}^{X*}U_{bj}^{Y*}(kc|aj)t_{ci}^{bk} = U_{ai}^{X*}U_{bj}^{Y*}B_{kc}^{Q}B_{aj}^{Q}U_{bk}^{Y'}U_{ci}^{X'}T_{X'Y'} = (U_{ai}^{X*}B_{aj}^{Q})(U_{ci}^{X'}B_{kc}^{Q})(U_{bj}^{Y*}U_{bk}^{Y'}T_{X'Y'}) = (U_{ai}^{X*}B_{aj}^{Q})(U_{ci}^{X'}B_{kc}^{Q})(U_{bk}^{Y'}T_{X'Y'})U_{bj}^{Y*} =$$

$$O(2N_{\mathrm{virt}}N_{\mathrm{occ}}^2N_{\mathrm{SVD}}N_{\mathrm{DF}} +N_{\mathrm{occ}}N_{\mathrm{virt}}N_{\mathrm{SVD}}^2 +2N_{\mathrm{virt}}N_{\mathrm{occ}}^2N_{\mathrm{SVD}}N_{\mathrm{DF}} +N_{\mathrm{virt}}N_{\mathrm{occ}}N_{\mathrm{SVD}}^2)$$

D2e(4) :

$$-U_{ai}^{X*}U_{bj}^{Y*}(kj|ac)t_{ci}^{bk} = -U_{ai}^{X*}U_{bj}^{Y*}B_{kj}^{Q}B_{ac}^{Q}U_{bk}^{Y'}U_{ci}^{X'}T_{X'Y'} = -(U_{ai}^{X*}B_{ac}^{Q}U_{ci}^{X'})(U_{bj}^{Y*}B_{kj}^{Q}U_{bk}^{Y'})T_{X'Y'}$$

$$O(2N_{\mathrm{virt}}^2N_{\mathrm{occ}}N_{\mathrm{SVD}}N_{\mathrm{DF}} +2N_{\mathrm{virt}}N_{\mathrm{occ}}N_{\mathrm{SVD}}^2N_{\mathrm{DF}} +N_{\mathrm{SVD}}^3N_{\mathrm{DF}} +N_{\mathrm{SVD}}^3N_{\mathrm{DF}})$$

D3a :

$$U_{ai}^{X*}U_{bj}^{Y*}(kc|ld)t_{ci}^{dj}t_{ak}^{bl} = U_{ai}^{X*}U_{bj}^{Y*}B_{kc}^{Q}B_{ld}^{Q}U_{dj}^{Y'}U_{ci}^{X'} U_{bl}^{Y''}U_{ak}^{X''}T_{X'Y'}T_{X''Y''} = (U_{ai}^{X*}U_{ak}^{X''})(U_{bj}^{Y*}U_{bl}^{Y''}T_{X''Y''}) (B_{kc}^{Q}U_{ci}^{X'}B_{ld}^{Q}U_{dj}^{Y'}T_{X'Y'}) = (U_{ai}^{X*}U_{ak}^{X''}\alpha_{ki}^{R})(U_{bj}^{Y*}U_{bl}^{Y''}\alpha_{lj}^{W})T_{X''Y''}o^{RW}$$

$$O(2N_{\mathrm{occ}}^2N_{\mathrm{virt}}N_{\mathrm{SVD}}^2 +2N_{\mathrm{occ}}^2N_{\mathrm{SVD}}^2N_{\mathrm{O}} +N_{\mathrm{O}}N_{\mathrm{SVD}}^3 +N_{\mathrm{O}}^2N_{\mathrm{SVD}}^2 +N_{\mathrm{SVD}}^3N_{\mathrm{O}})$$

D3b(1) :

$$U_{ai}^{X*}U_{bj}^{Y*}(kc|ld)t_{ai}^{ck}t_{bj}^{dl} = U_{ai}^{X*}U_{bj}^{Y*}B_{kc}^{Q}B_{ld}^{Q}U_{ck}^{Y'}U_{ai}^{X'} U_{bj}^{X''}U_{dl}^{Y''}T_{X'Y'}T_{X''Y''} = (B_{kc}^{Q}U_{ck}^{Y'}T_{XY'})(B_{ld}^{Q}U_{dl}^{Y''}T_{YY''})$$

$$O(2N_{\mathrm{occ}}N_{\mathrm{virt}}N_{\mathrm{SVD}}^2 +2N_{\mathrm{occ}}N_{\mathrm{virt}}N_{\mathrm{DF}}N_{\mathrm{SVD}} +N_{\mathrm{SVD}}^2N_{\mathrm{DF}})$$

D3b(2) :

$$-U_{ai}^{X*}U_{bj}^{Y*}(kd|lc)t_{ai}^{ck}t_{bj}^{dl} = -U_{ai}^{X*}U_{bj}^{Y*}B_{kd}^{Q}B_{lc}^{Q}U_{ck}^{Y'}U_{ai}^{X'} = U_{bj}^{X''}U_{dl}^{Y''}T_{X'Y'}T_{X''Y''} = -(B_{kd}^{Q}U_{dl}^{Y''}T_{YY''})(B_{lc}^{Q}U_{ck}^{Y'}T_{XY'})$$

$$O(2N_{\mathrm{occ}}N_{\mathrm{virt}}N_{\mathrm{SVD}}^2 +2N_{\mathrm{occ}}^2N_{\mathrm{virt}}N_{\mathrm{DF}}N_{\mathrm{SVD}} +N_{\mathrm{SVD}}^2N_{\mathrm{DF}})$$

D3b(3) :

$$\begin{aligned}
&U_{ai}^{X*}U_{bj}^{Y*}(kc|ld)t_{ci}^{ak}t_{dj}^{bl} = \\
&U_{ai}^{X*}U_{bj}^{Y*}B_{kc}^{Q}B_{ld}^{Q}U_{ak}^{Y'}U_{ci}^{X'} \\
&U_{bl}^{Y''}U_{dj}^{X''}T_{X'Y'}T_{X''Y''} = \\
&(B_{kc}^{Q}U_{ci}^{X'})(B_{ld}^{Q}U_{dj}^{X''})(U_{ai}^{X*}U_{ak}^{Y'}T_{X'Y'})(U_{bl}^{Y''}U_{bj}^{Y*}T_{X''Y''})
\end{aligned}
\qquad
\begin{aligned}
&O(2N_{\mathrm{occ}}^2N_{\mathrm{virt}}N_{\mathrm{DF}}N_{\mathrm{SVD}} \\
&+2N_{\mathrm{occ}}N_{\mathrm{virt}}N_{\mathrm{SVD}}^2 \\
&+2N_{\mathrm{occ}}^2N_{\mathrm{virt}}N_{\mathrm{SVD}}^2 \\
&+2N_{\mathrm{occ}}^2N_{\mathrm{SVD}}^2N_{\mathrm{DF}} \\
&+N_{\mathrm{SVD}}^2N_{\mathrm{DF}})
\end{aligned}$$

D3b(4) :

$$\begin{aligned}
&-U_{ai}^{X*}U_{bj}^{Y*}(kd|lc)t_{ci}^{ak}t_{dj}^{bl} = \\
&-U_{ai}^{X*}U_{bj}^{Y*}B_{kd}^{Q}B_{lc}^{Q}U_{ak}^{Y'}U_{ci}^{X'} \\
&U_{bl}^{Y''}U_{dj}^{X''}T_{X'Y'}T_{X''Y''} = \\
&-(U_{dj}^{X''}B_{kd}^{Q})(B_{lc}^{Q}U_{ci}^{X'})(U_{ai}^{X*}U_{ak}^{Y'})(U_{bj}^{Y*}U_{bl}^{Y''})T_{X'Y'}T_{X''Y''} = \\
&-(B_{kd}^{Q}U_{dj}^{X''}T_{X''Y''}B_{lc}^{Q}U_{bl}^{Y''})U_{bj}^{Y*}U_{ci}^{X'}(U_{ai}^{X*}U_{ak}^{Y'})T_{X'Y'} = \\
&(\beta_{kj}^{F}z^{FG}\beta_{bc}^{G})U_{bj}^{Y*}U_{ci}^{X'}(U_{ai}^{X*}U_{ak}^{Y'}T_{X'Y'})
\end{aligned}
\qquad
\begin{aligned}
&O(N_{\mathrm{occ}}^2N_{\mathrm{R}} \\
&+N_{\mathrm{occ}}^2N_{\mathrm{virt}}^2N_{\mathrm{R}} \\
&+N_{\mathrm{occ}}^2N_{\mathrm{virt}}^2N_{\mathrm{SVD}} \\
&+N_{\mathrm{occ}}N_{\mathrm{virt}}N_{\mathrm{SVD}}^2 \\
&+2N_{\mathrm{occ}}^2N_{\mathrm{virt}}N_{\mathrm{SVD}}^2 \\
&+N_{\mathrm{occ}}^2N_{\mathrm{SVD}}^3)
\end{aligned}$$

D3b(5) :

$$\begin{aligned}
&-P(ai|bj)U_{ai}^{X*}U_{bj}^{Y*}(kc|ld)t_{ai}^{ck}t_{dj}^{bl} = \\
&-P(X|Y)U_{ai}^{X*}U_{bj}^{Y*}B_{kc}^{Q}B_{ld}^{Q}U_{ck}^{Y'}U_{ai}^{X'} = \\
&U_{bl}^{Y''}U_{dj}^{X''}T_{X'Y'}T_{X''Y''} = \\
&-P(X|Y)(B_{kc}^{Q}U_{ck}^{Y'}T_{XY'})(B_{ld}^{Q}U_{dj}^{X''})(U_{bl}^{Y''}U_{bj}^{Y*}T_{X''Y''})
\end{aligned}
\qquad
\begin{aligned}
&O(N_{\mathrm{occ}}N_{\mathrm{virt}}N_{\mathrm{DF}}N_{\mathrm{SVD}} \\
&+N_{\mathrm{DF}}N_{\mathrm{SVD}}^2 \\
&+N_{\mathrm{occ}}^2N_{\mathrm{virt}}N_{\mathrm{DF}}N_{\mathrm{SVD}} \\
&+N_{\mathrm{occ}}N_{\mathrm{virt}}N_{\mathrm{SVD}}^2 \\
&+N_{\mathrm{occ}}^2N_{\mathrm{virt}}N_{\mathrm{SVD}}^2 \\
&+N_{\mathrm{occ}}^2N_{\mathrm{SVD}}^2N_{\mathrm{DF}} \\
&+N_{\mathrm{DF}}N_{\mathrm{SVD}}^2)
\end{aligned}$$

D3b(6) :

$$\begin{aligned}
&P(ai|bj)U_{ai}^{X*}U_{bj}^{Y*}(kd|lc)t_{ai}^{ck}t_{dj}^{bl} = \\
&P(X|Y)U_{ai}^{X*}U_{bj}^{Y*}B_{kd}^{Q}B_{lc}^{Q}U_{ck}^{Y'}U_{ai}^{X'} \\
&U_{bl}^{Y''}U_{dj}^{X''}T_{X'Y'}T_{X''Y''} = \\
&P(X|Y)(B_{lc}^{Q}U_{ck}^{Y'}T_{XY'})B_{kd}^{Q}U_{dj}^{X''}(U_{bj}^{Y*}U_{bl}^{Y''}T_{X''Y''}) =
\end{aligned}
\qquad
\begin{aligned}
&O(2N_{\mathrm{occ}}N_{\mathrm{virt}}N_{\mathrm{SVD}}^2 \\
&+2N_{\mathrm{occ}}^2N_{\mathrm{virt}}N_{\mathrm{DF}}N_{\mathrm{SVD}} \\
&+N_{\mathrm{occ}}^2N_{\mathrm{DF}}N_{\mathrm{virt}}N_{\mathrm{SVD}} \\
&+N_{\mathrm{occ}}^2N_{\mathrm{virt}}N_{\mathrm{SVD}}^2 \\
&+N_{\mathrm{occ}}N_{\mathrm{virt}}N_{\mathrm{SVD}}^2)
\end{aligned}$$

D3c(1) :

$$\begin{aligned}
&P(ai|bj)U_{ai}^{X*}U_{bj}^{Y*}(kc|ld)t_{cj}^{dk}t_{ai}^{bl} = \\
&P(X|Y)U_{ai}^{X*}U_{bj}^{Y*}B_{kc}^{Q}B_{ld}^{Q}U_{dk}^{Y'}U_{cj}^{X'} \\
&U_{bl}^{Y''}U_{ai}^{X''}T_{X'Y'}T_{X''Y''} = \\
&P(X|Y)(B_{kc}^{Q}U_{cj}^{X'}T_{X'Y'})(B_{ld}^{Q}U_{dk}^{Y'})(U_{bj}^{Y*}U_{bl}^{Y''}T_{XY''})
\end{aligned}
\qquad
\begin{aligned}
&O(2N_{\mathrm{occ}}N_{\mathrm{virt}}N_{\mathrm{SVD}}^2 \\
&+N_{\mathrm{occ}}^2N_{\mathrm{virt}}N_{\mathrm{DF}}N_{\mathrm{SVD}} \\
&+N_{\mathrm{occ}}^2N_{\mathrm{virt}}N_{\mathrm{SVD}}^2 \\
&+N_{\mathrm{occ}}^2N_{\mathrm{virt}}N_{\mathrm{DF}}N_{\mathrm{SVD}} \\
&+N_{\mathrm{occ}}^3N_{\mathrm{SVD}}N_{\mathrm{DF}} \\
&+N_{\mathrm{occ}}^2N_{\mathrm{SVD}}^2)
\end{aligned}$$

D3c(2) :

$$\begin{aligned}
&-P(ai|bj)U_{ai}^{X*}U_{bj}^{Y*}(kd|lc)t_{cj}^{dk}t_{ai}^{bl} = \\
&-P(X|Y)U_{ai}^{X*}U_{bj}^{Y*}B_{kd}^{Q}B_{lc}^{Q}U_{dk}^{Y'}U_{cj}^{X'} \\
&U_{bl}^{Y''}U_{ai}^{X''}T_{X'Y'}T_{X''Y''} = \\
&-P(X|Y)(B_{kd}^{Q}U_{dk}^{Y'})(B_{lc}^{Q}U_{cj}^{X'}T_{X'Y'})(U_{bj}^{Y*}U_{bl}^{Y''}T_{XY''})
\end{aligned}
\qquad
\begin{aligned}
&O(2N_{\mathrm{occ}}N_{\mathrm{virt}}N_{\mathrm{SVD}}^2 \\
&+N_{\mathrm{occ}}^2N_{\mathrm{virt}}N_{\mathrm{DF}}N_{\mathrm{SVD}} \\
&+N_{\mathrm{occ}}^2N_{\mathrm{virt}}N_{\mathrm{SVD}}^2 \\
&+N_{\mathrm{occ}}^2N_{\mathrm{virt}}N_{\mathrm{DF}}N_{\mathrm{SVD}} \\
&+N_{\mathrm{occ}}^3N_{\mathrm{SVD}}N_{\mathrm{DF}} \\
&+N_{\mathrm{occ}}^2N_{\mathrm{SVD}}^2)
\end{aligned}$$

$$
\text{D3d(1)}: \quad \begin{aligned} -P(ai|bj)U_{ai}^{X*}U_{bj}^{Y*}(kc|ld)t_{ck}^{al}t_{di}^{bj} = \\ -P(X|Y)U_{ai}^{X*}U_{bj}^{Y*}B_{kc}^{Q}B_{ld}^{Q}U_{al}^{Y'}U_{ck}^{X'} \\ U_{bj}^{Y''}U_{di}^{X''}T_{X'Y'}T_{X''Y''} = \\ -P(X|Y)(B_{kc}^{Q}U_{ck}^{X'}T_{X'Y'})(B_{ld}^{Q}U_{di}^{X''}T_{X''Y})(U_{ai}^{X*}U_{al}^{Y'}) \end{aligned} \quad \begin{aligned} O(2N_{\text{occ}}N_{\text{virt}}N_{\text{SVD}}^{2} \\ +N_{\text{occ}}^{2}N_{\text{virt}}N_{\text{DF}}N_{\text{SVD}} \\ +N_{\text{occ}}N_{\text{virt}}N_{\text{DF}}N_{\text{SVD}} \\ +N_{\text{occ}}^{2}N_{\text{virt}}N_{\text{SVD}}^{2} \\ +N_{\text{occ}}^{2}N_{\text{SVD}}^{2}N_{\text{DF}} \\ +N_{\text{occ}}^{2}N_{\text{DF}}N_{\text{SVD}}^{2}) \end{aligned}
$$

$$
\text{D3d(2)}: \quad \begin{aligned} P(ai|bj)U_{ai}^{X*}U_{bj}^{Y*}(kd|lc)t_{ck}^{al}t_{di}^{bj} = \\ P(X|Y)U_{ai}^{X*}U_{bj}^{Y*}B_{kd}^{Q}B_{lc}^{Q}U_{al}^{Y'}U_{ck}^{X'} \\ U_{bj}^{Y''}U_{di}^{X''}T_{X'Y'}T_{X''Y''} = \\ P(X|Y)(B_{kd}^{Q}U_{di}^{X''}T_{X''Y})(B_{lc}^{Q}U_{ck}^{X'}T_{X'Y'})U_{al}^{Y'}U_{ai}^{X*} \end{aligned} \quad \begin{aligned} O(2N_{\text{occ}}N_{\text{virt}}N_{\text{SVD}}^{2} \\ +2N_{\text{occ}}^{2}N_{\text{virt}}N_{\text{DF}}N_{\text{SVD}} \\ +N_{\text{occ}}^{2}N_{\text{SVD}}N_{\text{DF}}N_{\text{virt}} \\ +N_{\text{occ}}^{2}N_{\text{DF}}N_{\text{virt}}N_{\text{SVD}} \\ +N_{\text{occ}}N_{\text{R}}N_{\text{SVD}}^{2}) \end{aligned}
$$

## MOLECULAR GEOMETRIES AND BASIS SETS FOR GOLD CLUSTERS AND GOLD (I) CHLORIDE

Molecular geometries are taken from:

- $(AuCl)_n$ chains: [2]
- $Au_2$ molecule: [3]
- $Au_3$ molecule: [4]
- $Au_4$, $Au_5$ molecules: [5]

For a basis set the NWChem-style format is assumed [6, 7].

```
#
# geometries: (AuCl)_n
# units: angstroms
#

# AuCl
Au   0.0000   0.0000   0.0000
Cl   0.0000   0.0000   2.3559

# (AuCl)2
Cl  -1.6835  -1.6481   0.0000
Au   0.0000   0.0000   0.0000
Cl   1.6835   1.6481   0.0000
Au   3.3670   0.0000   0.0000

# (AuCl)3
Cl  -1.6835  -1.6481   0.0000
Au   0.0000   0.0000   0.0000
Cl   1.6835   1.6481   0.0000
Au   3.3670   0.0000   0.0000
Cl   5.0505  -1.6481   0.0000
Au   6.7340   0.0000   0.0000

#
# geometries: Au_n
# units: angstroms
#

# Au2
Au   0.0000   0.0000   0.0000
Au   0.0000   0.0000   2.4720

# Au3
Au   0.0000   0.0000   0.0000
Au   0.0000   0.0000   2.6334
Au   2.2806   0.0000   1.3167

# Au4
Au   0.0000   0.0000   2.3118
Au   0.0000   1.2961   0.0000
Au   0.0000  -1.2961   0.0000
Au   0.0000   0.0000  -2.3118
```

```
# Au5
Au   0.0000   1.3269  -1.4006
Au   0.0000   2.5896   0.9114
Au   0.0000   0.0000   0.9785
Au   0.0000  -1.3269  -1.4006
Au   0.0000  -2.5896   0.9113

basis
Au S
  1.2354184E+01 -0.02274581 -0.00877638 -0.02555932  0.03693972  0.01573320
  7.5641217E+00 -0.32030040 -0.12836585 -0.24756589  0.52005059  1.31813528
  4.5739925E+00  1.22730988  0.52999848  1.09809463 -2.45619107 -7.15394004
  2.7396490E+00 -0.39602850 -0.24516616 -0.29506137  1.12929477 11.26180779
  1.5458697E+00 -0.55003023 -0.22604847 -1.27783285  5.08760499 -3.45494579
  8.5989884E-01 -0.62756592 -0.43315933 -0.85382166 -5.32545532 -8.26261961
  4.5826151E-01 -0.08731456 -0.05413855  1.50970855 -0.93181824 10.92918166
  2.4308744E-01 -0.03222277  0.20449165  1.06615995  2.75181865 -4.49742365
  1.2152573E-01  0.01348855  0.55608044 -0.40883856  0.26298930 -1.19295738
  6.0893308E-02 -0.00840686  0.38745650 -0.73754090 -0.96373842  1.09501336
  3.0185296E-02  0.00462417  0.09191093 -0.10610295 -0.12975976  0.30194584
  1.5092648E-02 -0.00205445 -0.00713047 -0.00570219 -0.00807426 -0.04542742
  7.5463240E-03  0.00051764  0.00202094  0.00136140  0.00218376  0.01050147
Au P
  8.8298688E+00  0.02935292  0.01422975  0.10585760  0.19404095 -0.41789073  1.11065916
  4.9910401E+00 -0.29527114  0.48165800  0.65231246  0.52739910  0.02131160 -3.35743544
  2.7579796E+00  0.13137000 -1.01620687 -2.37219180 -3.37941109  4.25707765  2.61925752
  1.5021522E+00  0.55369630 -0.15917122  1.06358754  3.81689577 -8.90054258  1.87126694
  8.0099970E-01  0.38005164 -0.14428549  0.57492315 -0.64027484  8.72083932 -6.61987955
  4.1615897E-01  0.15772293  0.72442889  0.37046304 -1.40508464 -4.15402329  7.82125107
  1.8857106E-01  0.00416543  0.31978470 -0.94217463  0.18901851  0.15166921 -6.11125386
  8.7555118E-02  0.00538095  0.09649488 -0.07393741  0.88758831  0.57900323  3.32772240
  4.0633898E-02 -0.00311073 -0.01437783 -0.08759176 -0.11823203  0.20449586 -0.94088477
  1.8755275E-02  0.00153408  0.00822088  0.03846490  0.07550931 -0.06424161  0.55237581
  8.7233837E-03 -0.00046462 -0.00246712 -0.01163687 -0.02262144  0.01902742 -0.16732817
Au D
  2.3402974E+01   0.00070504  0.00219000 -0.00176954 -0.02107128  0.06913875
  1.3090124E+01   0.00065896 -0.00491021  0.00178971  0.09455013 -0.33105461
  7.2436307E+00   0.02071924  0.05025369 -0.04493545 -0.35692279  1.10150541
  3.9591472E+00   0.03393130  0.02354993 -0.09371798  0.37236468 -2.08031609
  2.0937190E+00  -0.20686565 -0.42441503  0.83658602  1.46683440  0.61306514
  1.0655856E+00  -0.37731570 -0.48026132  0.04741036 -2.07301100  1.94934640
  5.1928944E-01  -0.35791026  0.17829416 -1.03167700  0.45084647 -3.10238927
  2.3993836E-01  -0.22819910  0.57022364  0.12524451  0.96532664  2.36696282
  1.0271158E-01  -0.06005416  0.27057818  0.69642655 -0.71335753 -0.77262154
  4.6265062E-02  -0.00169308  0.01928482  0.11210968 -0.18831774 -0.27780691
Au F
  5.6535919E+01  -0.00007981 -0.00174761
  3.0055120E+01   0.00011911  0.00731866
  1.6265242E+01  -0.00082227 -0.02036960
  8.7169377E+00  -0.00000334  0.03976438
  4.5407487E+00  -0.02241108 -0.13161976
  2.2220809E+00   0.18163627  0.64708458
  9.6965516E-01   0.57045653  0.36370688
  3.8700265E-01   0.39887128 -0.76465739
  1.5480106E-01   0.04380496 -0.21484707
  6.1920424E-02   0.00650312 -0.01263902
```

```
Au G
  8.0000          0.01369021
  3.2000          0.10097062
  1.2800          0.64198482
  0.5120          0.40866881
  0.2048          0.03172163
end

basis
Cl S
 935.41546    0.0012890240   0.0004259894   0.0  0.0
 128.06385    0.0167050108   0.0057967467   0.0  0.0
  30.44428    0.1978014762   0.0712977391   0.0  0.0
  21.14379   -0.0234641142  -0.0132311291   0.0  0.0
   6.33400   -0.4976201485  -0.2049752614   0.0  0.0
   2.69400   -0.5630761636  -0.4065425096   0.0  0.0
   0.97680   -0.0741893792   0.0847991034   1.0  0.0
   0.43130    0.0067764551   0.7241386451   0.0  0.0
   0.16250   -0.0018790722   0.3902205075   0.0  1.0
Cl P
 690.16986   -0.0024275485  -0.0633109750   0.0006559181  0.0  0.0
 160.58286   -0.0191359393  -0.1506152380   0.0051602356  0.0  0.0
  50.59551   -0.0886356051  -0.3196798411   0.0246436873  0.0  0.0
  18.53149   -0.2564811125  -0.4213031493   0.0727522005  0.0  0.0
   7.25609   -0.4380669231  -0.1158467636   0.1341030088  0.0  0.0
   2.92200   -0.3498840600   0.5951399503   0.0943930451  0.0  0.0
   1.02200   -0.0579603360   0.3003928008  -0.2626977294  1.0  0.0
   0.38180    0.0044666713  -0.0303502205  -0.5640809277  0.0  0.0
   0.13010   -0.0022263633   0.0147021065  -0.3415007020  0.0  1.0
Cl D
   1.04600   1.0
Cl D
   0.34400   1.0
Cl F
   0.70600   1.0
end
```

## CLUSTER MODEL OF YTTERBIUM (II) CHLORIDE

Cluster model obtained within the CTEP approach consists of [8–12]:

- Cartesian coordinates of all main-cluster atoms, pseudoatoms of nearest cation (NCE) and anion (NAE) environment layers and additional fractional point charges placed at these pseudoatoms;
- Basis sets and relativistic pseudopotentials for the main-cluster atoms;
- Auxuliary basis sets and compound-tunable pseudopotentials (CTPPs) for pseudoatoms of NCE and NAE layers.

For basis sets and pseudopotentials the NWChem-style format is assumed [6, 7].

```
# units: angstroms
# main cluster
#                      x               y               z
Yb             1.5261119935    5.0463003255    0.3201010786
Cl             0.0151468446    6.0788334177   -1.8688676495
Cl             2.2355019096    3.9017948504    2.7632273525
Cl            -1.0976310929    3.9017948504    0.7433128654
```

```
Cl             2.2355019096    2.5943891846   -0.7433128654
Cl            -0.0151468446    6.9135346524    1.8688676495
Cl             3.3179861579    6.9135346524    1.6376725684
Cl             3.3482798472    6.0788334177   -1.6376725684

# nearest cation environment
#                   x               y               z
Yb            -1.8070210090    5.0463003255   -3.8266412964
Yb             1.8070210090    7.9460677447   -3.1864391393
Yb            -1.5261119935    7.9460677447   -0.3201010786
Yb             1.5261119935    1.4498837096    3.8266412964
Yb             4.8592449960    5.0463003255    3.1864391393
Yb            -1.8070210090    1.4498837096   -0.3201010786
Yb            -1.8070210090    5.0463003255    3.1864391393
Yb             1.5261119935    1.4498837096   -3.1864391393
Yb             4.8592449960    1.4498837096   -0.3201010786
Yb             1.8070210090    7.9460677447    3.8266412964
Yb             5.1401540116    7.9460677447   -0.3201010786
Yb             4.8592449960    5.0463003255   -3.8266412964

# additional fractional charges (simulating NAE)
#     q             x               y               z
 1.30805219   -1.8070210090    5.0463003255   -3.8266412964
 1.44132923    1.8070210090    7.9460677447   -3.1864391393
 1.44515204   -1.5261119935    7.9460677447   -0.3201010786
 1.32343555    1.5261119935    1.4498837096    3.8266412964
 1.45385552    4.8592449960    5.0463003255    3.1864391393
 1.11176582   -1.8070210090    1.4498837096   -0.3201010786
 1.58729059   -1.8070210090    5.0463003255    3.1864391393
 0.91160661    1.5261119935    1.4498837096   -3.1864391393
 1.10687524    4.8592449960    1.4498837096   -0.3201010786
 1.66079001    1.8070210090    7.9460677447    3.8266412964
 1.50846236    5.1401540116    7.9460677447   -0.3201010786
 1.02752333    4.8592449960    5.0463003255   -3.8266412964
-0.04076774   -4.4307640955    3.9017948504   -4.2498530832
-0.28597253   -3.3482798472    6.9135346524   -5.3754078673
-0.00018281   -1.0976310929    3.9017948504   -6.2697675704
-0.41028287   -3.3179861579    6.0788334177   -1.6376725684
-0.21328770   -1.0976310929    2.5943891846   -2.7632273525
-0.54032671   -0.0151468446    6.9135346524   -5.1442127862
-0.17555236    3.3179861579    6.9135346524   -5.3754078673
-0.23979709    1.0976310929   10.3979788855   -4.2498530832
-0.00000000    1.0976310929    9.0905732197   -0.7433128654
-0.62700000    4.4307640955    9.0905732197   -2.7632273525
-0.43958472   -3.3482798472    6.9135346524    1.6376725684
-0.19666401   -2.2355019096   10.3979788855    0.7433128654
-0.60401553   -2.2355019096    9.0905732197   -2.7632273525
-0.53033235    0.0151468446    0.4173506174    1.6376725684
-0.14748401    3.3179861579   -0.4173506174    5.1442127862
-0.11742628   -0.0151468446   -0.4173506174    5.3754078673
-0.18219029   -1.0976310929    2.5943891846    4.2498530832
-0.08998141    2.2355019096    2.5943891846    6.2697675704
-0.23259687    3.3482798472    0.4173506174    1.8688676495
-0.19111472    5.5686349122    3.9017948504    0.7433128654
-0.21959169    3.3482798472    6.0788334177    5.3754078673
-0.26869876    6.6814128497    6.0788334177    5.1442127862
```

```
-0.22565882     5.5686349122     2.5943891846     4.2498530832
-0.61663843     6.6511191605     6.9135346524     1.8688676495
 0.00000000    -3.3482798472    -0.4173506174    -1.8688676495
 0.00000000    -4.4307640955     2.5943891846    -0.7433128654
-0.15031786    -0.0151468446    -0.4173506174    -1.6376725684
-0.11242661    -3.3179861579     0.4173506174     1.8688676495
-0.00000000    -4.4307640955     3.9017948504     2.7632273525
-0.45105764    -3.3179861579     6.0788334177     5.3754078673
-0.53985613     0.0151468446     6.0788334177     5.1442127862
 0.00000000     0.0151468446     0.4173506174    -5.3754078673
-0.10562518     2.2355019096     3.9017948504    -4.2498530832
 0.00000000     3.3179861579    -0.4173506174    -1.8688676495
-0.27005531     3.3482798472     0.4173506174    -5.1442127862
-0.23338520     6.6814128497     0.4173506174     1.6376725684
-0.11260783     6.6511191605    -0.4173506174    -1.6376725684
-0.33081834     5.5686349122     2.5943891846    -2.7632273525
-0.32565057     1.0976310929    10.3979788855     2.7632273525
-0.31068798     1.0976310929     9.0905732197     6.2697675704
-0.41350967     4.4307640955     9.0905732197     4.2498530832
-0.32668224     6.6814128497     6.0788334177    -1.8688676495
-0.27370639     7.7638970980     9.0905732197    -0.7433128654
-0.10798809     4.4307640955    10.3979788855     0.7433128654
 0.00000000     5.5686349122     3.9017948504    -6.2697675704
-0.22657574     6.6511191605     6.9135346524    -5.1442127862


# ytterbium (main cluster)

basis
Yb S
  5.6622900000     -0.23956340000
  3.0558900000      0.89349670000
  1.0772600000     -0.69801440000
Yb S
 0.44751000000      1.0
Yb S
 0.29834000000      1.0
Yb S
 0.13260000000      1.0
Yb P
  4.0772800000      0.91496100000E-01
  3.3977300000     -0.24947820000
 0.78282000000      0.41128460000
Yb P
  1.6460600000      1.0
Yb P
 0.34423000000      1.0
Yb P
 0.13929000000      1.0
Yb D
 0.61623000000      1.0
Yb D
 0.18155000000      1.0
Yb F
  1.0285100000      1.0
Yb F
```

```
 0.31000000000      1.0
end

#
# 10e-GRECP for Yb
# by N.S.Mosyagin, 03.07.15
# taking into account the contributions from Breit interactions and finite nuclear size
# Pseudospinors from the [4s^2 4p^6 4d^10 4f^14] 5s^2 5p^6 6s^0.4 5d^0.3 6p^0.3 state
#
# http://www.qchem.pnpi.spb.ru/data/files/Yb.zip
#

# chlorine (main cluster)

basis
Cl S
  69507.990945      0.54314897497E-03
  10426.156880      0.41990463961E-02
  2373.2334061      0.21592141679E-01
  671.56420071      0.84598850094E-01
  218.41999790      0.24757249724
  77.572249714      0.47016930228
  28.888815277      0.37436370716
Cl S
  127.10527185      0.25182166603E-01
  39.339582961      0.10786112456
  7.6740679989     -0.27408821574
Cl S
  3.8745627630       1.3213875014
  1.8385832573      0.68636955368
Cl S
 0.44985945000      1.0
Cl S
 0.13637031000      1.0
Cl P
  666.50423284      0.23632663836E-02
  157.64241690      0.18879300374E-01
  50.262520978      0.87206341273E-01
  18.536078105      0.25285612970
  7.2940532777      0.43507154820
Cl P
  2.8014916400      1.0
Cl P
 0.73964278000      1.0
Cl P
 0.21056105000      1.0
Cl D
 0.23728440000      1.0
end

# pseudo-ytterbium (NCE)

basis
Yb S
  1.7033531779      0.32943044601E-01
 0.35945519359     -0.47770335258
```

```
Yb S
 0.29834000000      1.0
Yb S
 0.13260000000      1.0
Yb P
 0.29220769175     -0.20166527403
 0.14692241953      0.97860710742E-01
Yb P
 0.13929000000      1.0
Yb D
  2.3929791237     -0.13914446181E-01
 0.82537127393      0.27628167053
 0.28468185664      0.54161642333
Yb D
 0.18155000000      1.0
end

#
# 2e-RECP for the Yb +1.8 cation, 4 gaussians per l,
# without SO interactions, by N.S.Mosyagin from 19.10.18
# Pseudospinors from the 4s^0.15 4p^0.025 3d^0.025 state,
# 5-4-3 gaussians per l
#

ecp
Yb nelec 18
Yb UL
 1   12.1426975      -15.2386012
 1    3.6608059      -14.5775174
 1    0.9869034       -7.9349017
 1    0.3559306       -0.8397914
Yb S
 0    0.1198414       10.0000000
 1    8.2657933       22.7174604
 1    1.4990175       11.7793783
 2    0.1876474       -2.0249546
Yb P
 0    0.2757268        9.0000000
 1    9.9771245       19.3438417
 1    2.3035432       13.5516361
 1    0.5285219        3.1375203
Yb D
 0    2.5235783        7.0000000
 1    9.9798004       14.8276980
 1    2.2132429       15.4139348
 1    0.1344036       -0.2753461
Yb F
 0    0.2267468        4.0000000
 1   12.1426975       15.2386012
 1    3.6608059       14.5775174
 1    0.9869034        7.9349017
 1    0.3559306        0.8397914
end
```

[1] I. Shavitt and R. J. Bartlett, *Many-Body Methods in Chemistry and Physics: MBPT and Coupled-Cluster Theory*, Cambridge Molecular Science (Cambridge University Press, 2009).
[2] E. M. W. Janssen, J. C. W. Folmer, and G. A. Wiegers, The preparation and crystal structure of gold monochloride, AuCl, Journal of the Less Common Metals **38**, 71–76 (1974).
[3] G. A. Bishea and M. D. Morse, Spectroscopic studies of jet-cooled AgAu and $Au_2$, J. Chem. Phys. **95**, 5646–5659 (1991).
[4] A. A. Rusakov, Comment on "Potential energy surface of group 11 trimers (Cu, Ag, Au): Bond angle isomerism in $Au_3$", J. Phys. Chem. A **127**, 7673–7675 (2023).
[5] H. Baek, J. Moon, and J. Kim, Benchmark study of density functional theory for neutral gold clusters, $Au_n$ ($n = 2 - 8$), J. Phys. Chem. A **121**, 2410–2419 (2017).
[6] (2025), NWChem: Open Source High-Performance Computational Chemistry. Basis sets. `https://nwchemgit.github.io/Basis.html` (accessed on 7 June 2025).
[7] (2025), NWChem: Open Source High-Performance Computational Chemistry. Effective Core Potentials. `https://nwchemgit.github.io/ECP.html` (accessed on 7 June 2025).
[8] Y. V. Lomachuk, D. A. Maltsev, N. S. Mosyagin, L. V. Skripnikov, R. V. Bogdanov, and A. V. Titov, Compound-tunable embedding potential: which oxidation state of uranium and thorium as point defects in xenotime is favorable?, Phys. Chem. Chem. Phys. **22**, 17922–17931 (2020).
[9] D. A. Maltsev, Y. V. Lomachuk, V. M. Shakhova, N. S. Mosyagin, L. V. Skripnikov, and A. V. Titov, Compound-tunable embedding potential method and its application to calcium niobate crystal $CaNb_2O_6$ with point defects containing tantalum and uranium, Phys. Rev. B **103**, 205105 (2021).
[10] V. M. Shakhova, D. A. Maltsev, Y. V. Lomachuk, N. S. Mosyagin, L. V. Skripnikov, and A. V. Titov, Compound-tunable embedding potential method: analysis of pseudopotentials for Yb in $YbF_2$, $YbF_3$, $YbCl_2$ and $YbCl_3$ crystals, Phys. Chem. Chem. Phys. **24**, 19333–19345 (2022).
[11] D. A. Maltsev, Y. V. Lomachuk, V. M. Shakhova, N. S. Mosyagin, D. O. Kozina, and A. V. Titov, Electronic structure study of $YNbTiO_6$ vs. $CaNb_2O_6$ with U, Pu and minor actinide substitutions using compound-tunable embedding potential method (2023), arXiv:2310.20595 [cond-mat.mtrl-sci].
[12] A. V. Oleynichenko, Y. V. Lomachuk, D. A. Maltsev, N. S. Mosyagin, V. M. Shakhova, A. Zaitsevskii, and A. V. Titov, Compound-tunable embedding potential method to model local electronic excitations on $f$-element ions in solids: pilot relativistic coupled cluster study of Ce and Th impurities in yttrium orthophosphate, $YPO_4$, Phys. Rev. B **109**, 125106 (2024).
